# Supplementary material for: Bayesian Non-parametric Quantile Process Regression and Estimation of Marginal Quantile Effects
Source: arXiv:2102.11309 source file (2021-08-29)

**Simulation 1**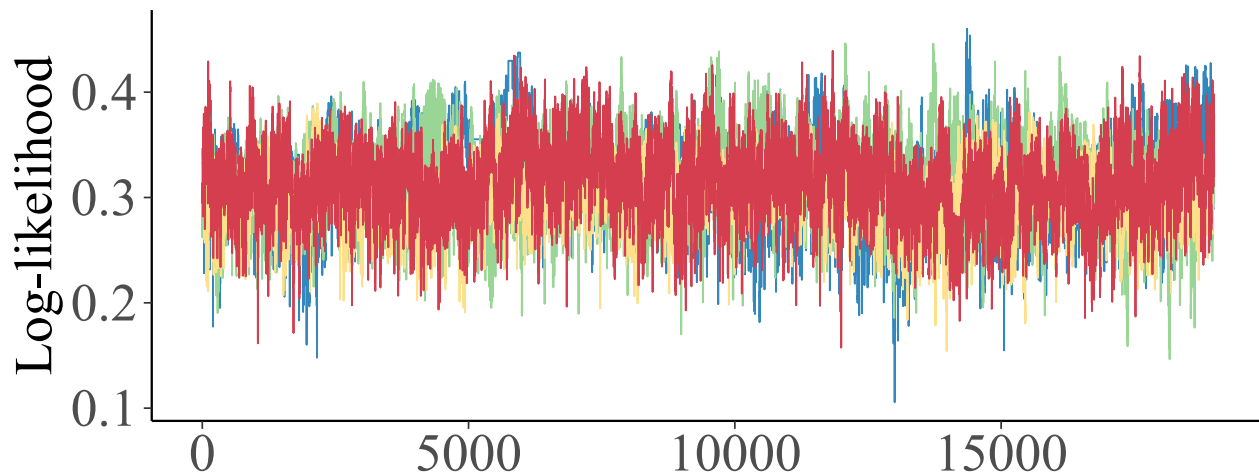**Simulation 2**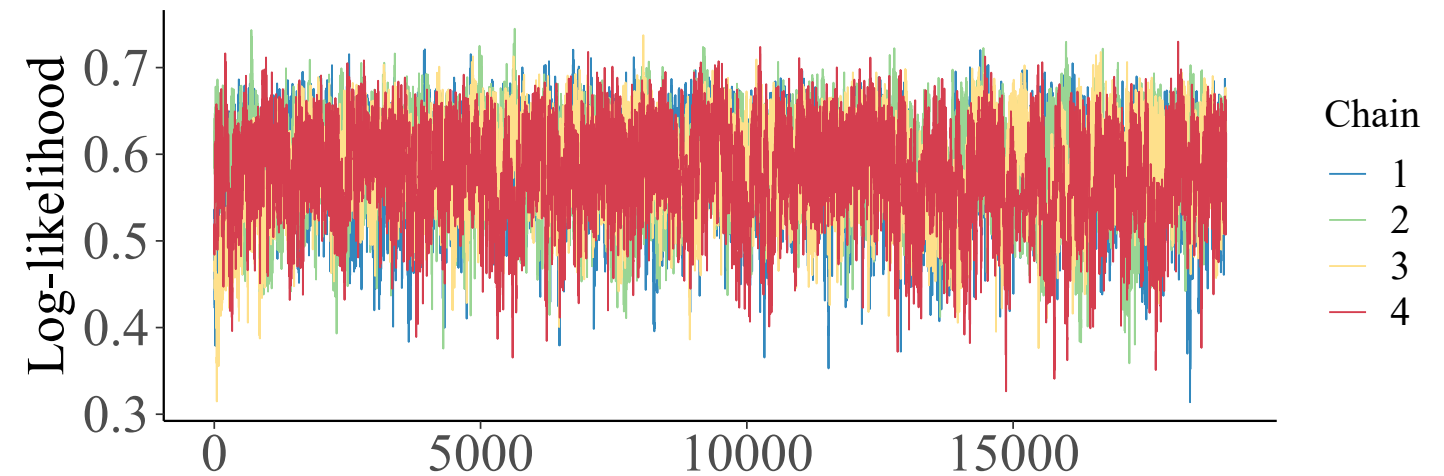**Simulation 3**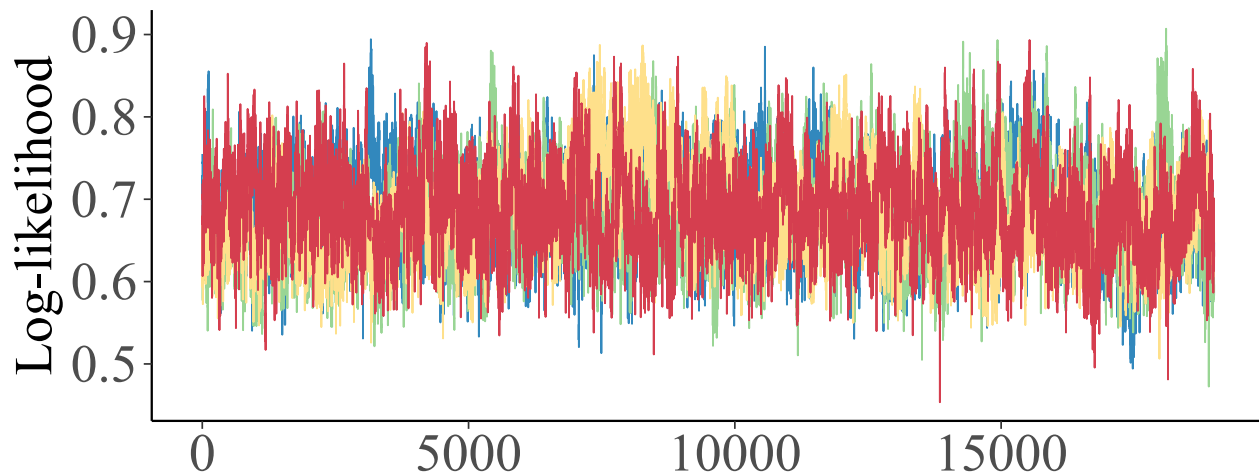**Simulation 4**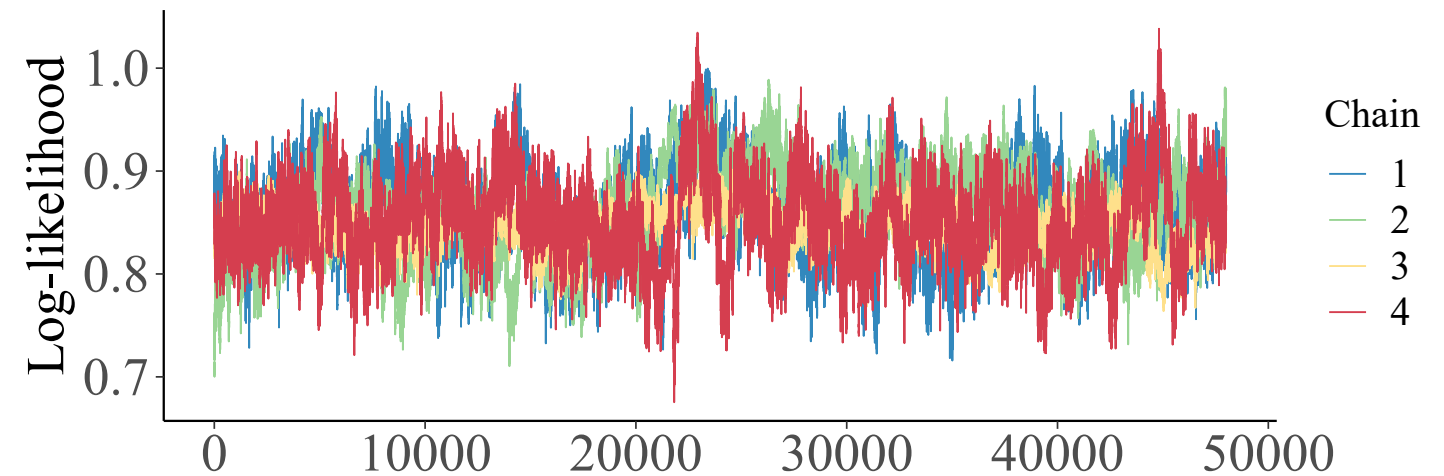

### Simulation 1

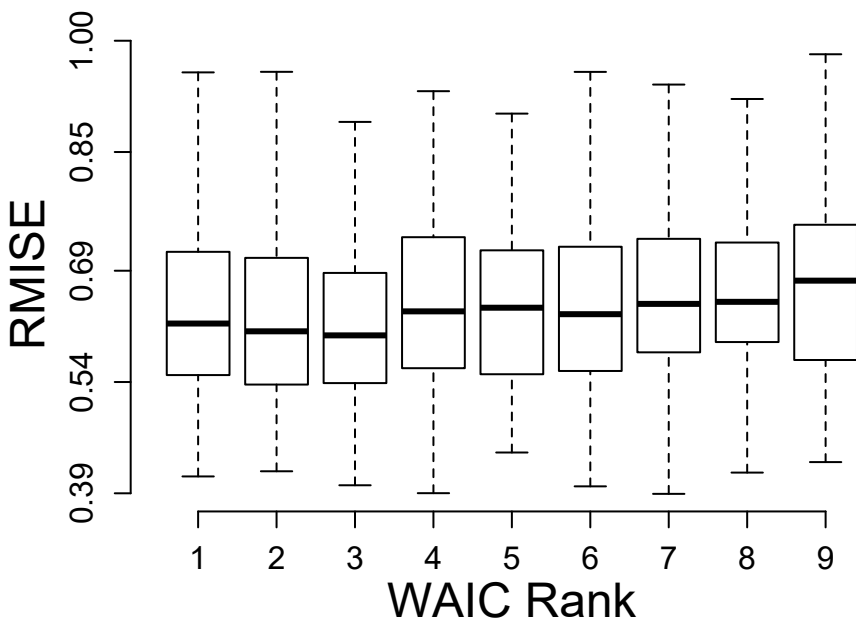

### Simulation 2

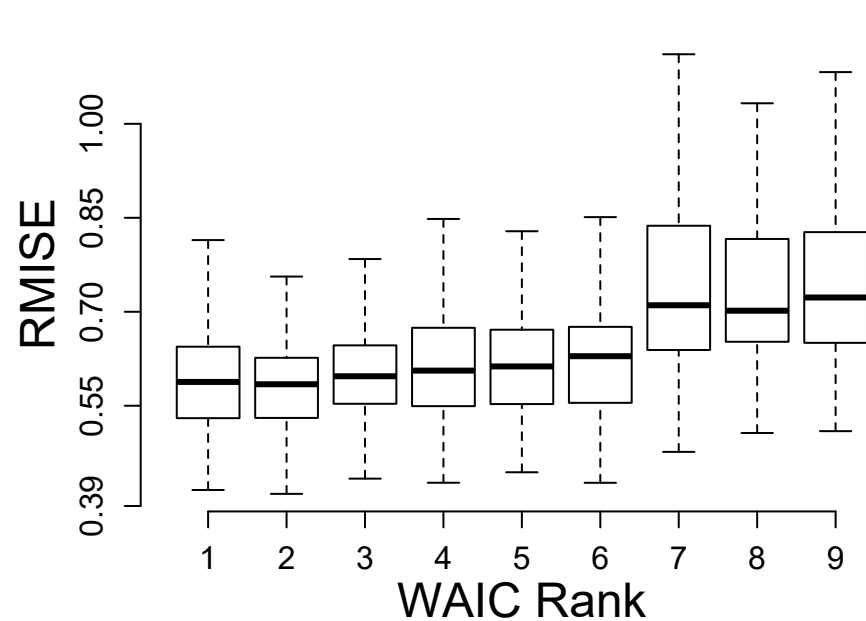

### Simulation 3

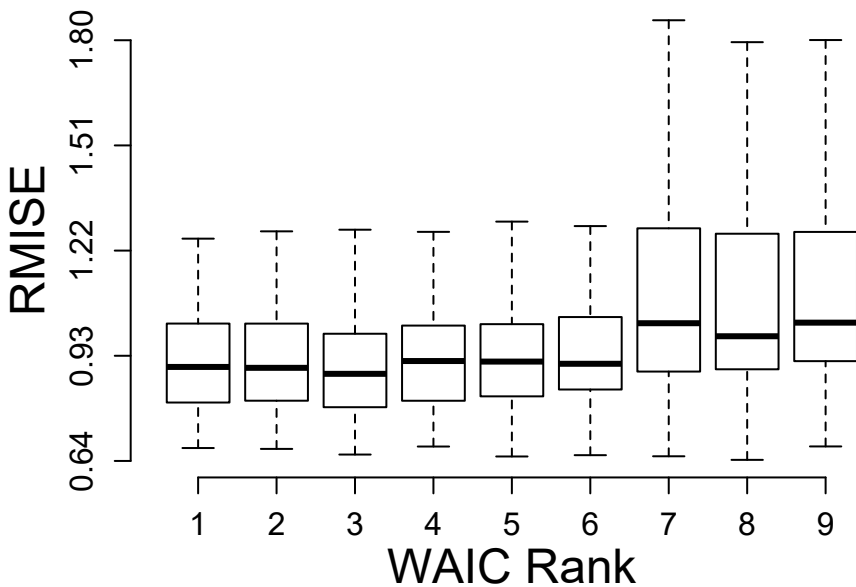

### Simulation 4

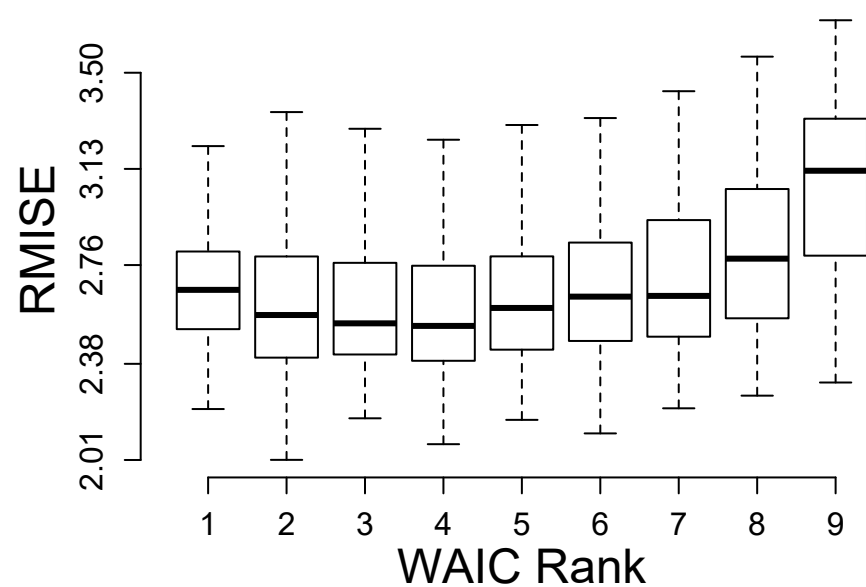

# Estimated Quantiles

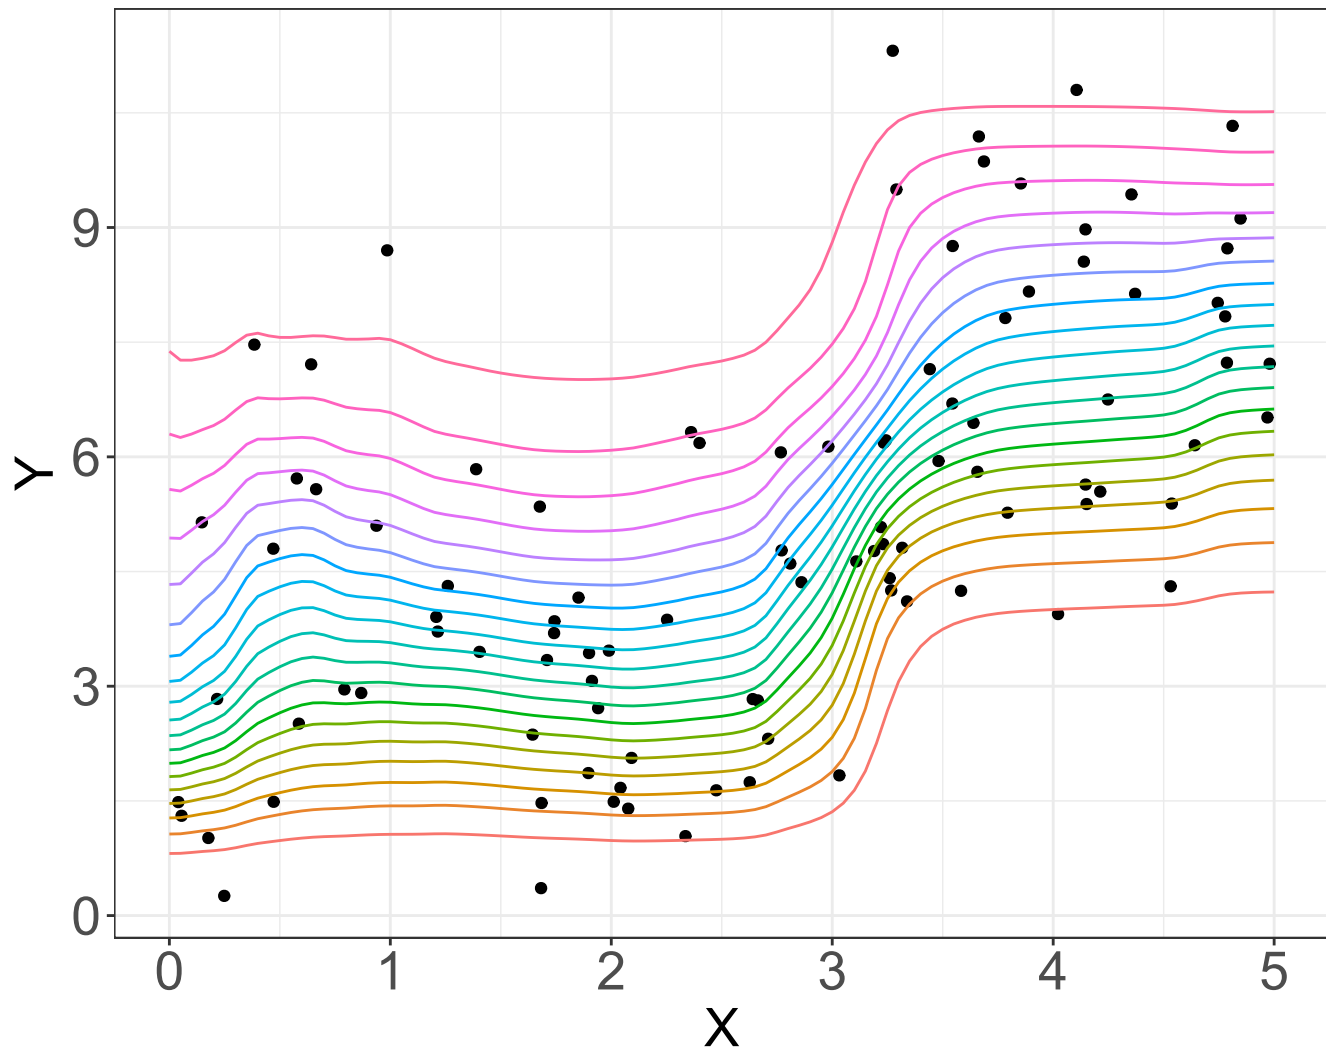

*Estimated Density at  $X = 0.5$*

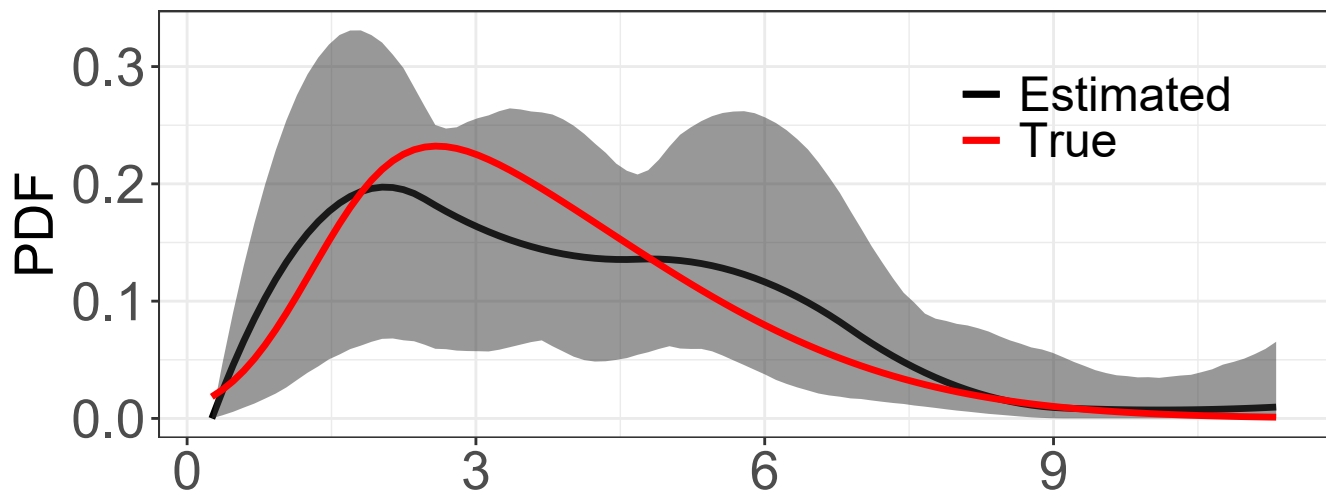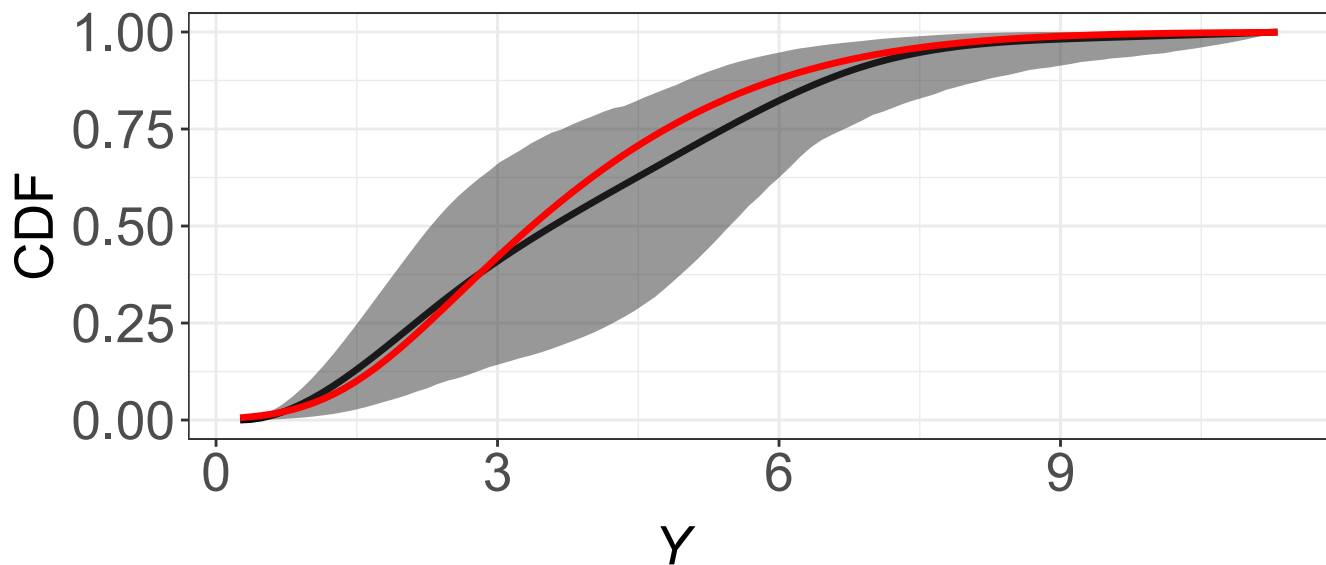

*Estimated Density at  $X = 2$*

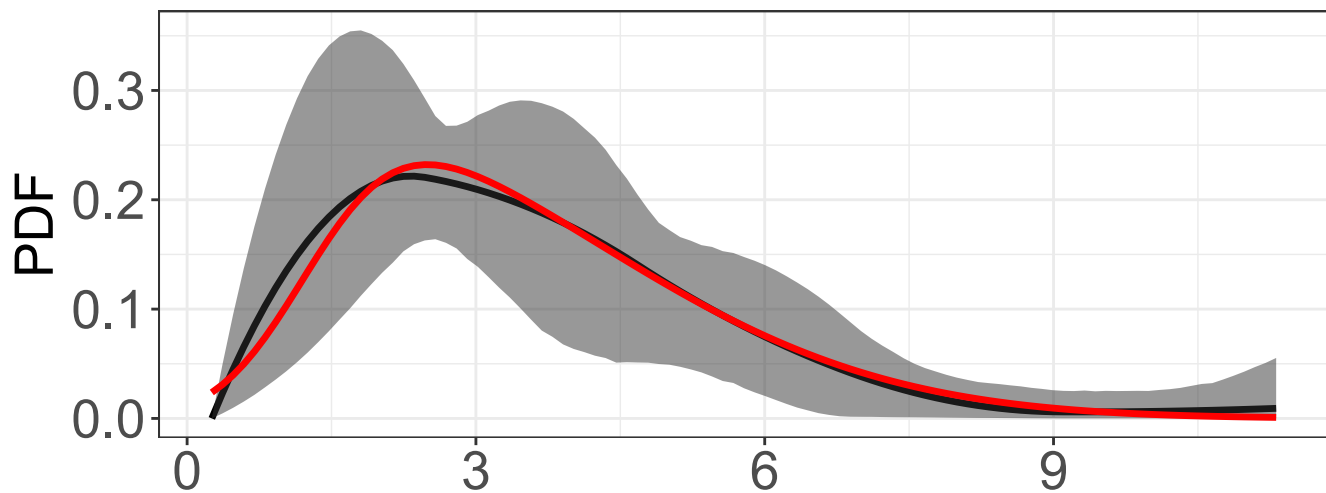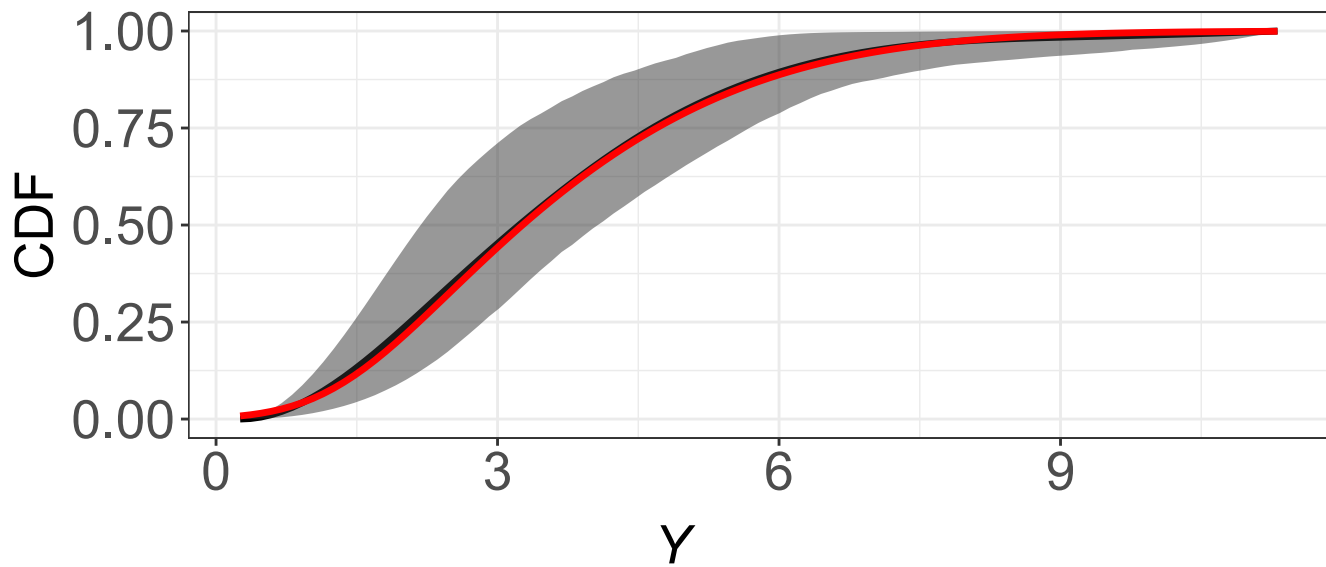

*Estimated Density at  $X = 3.5$*

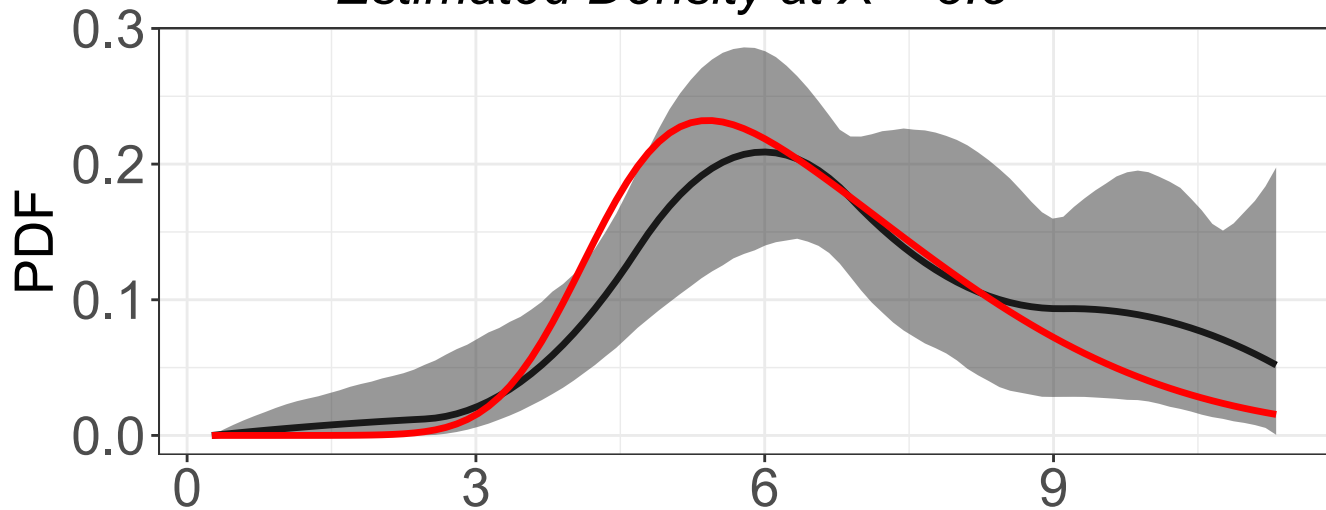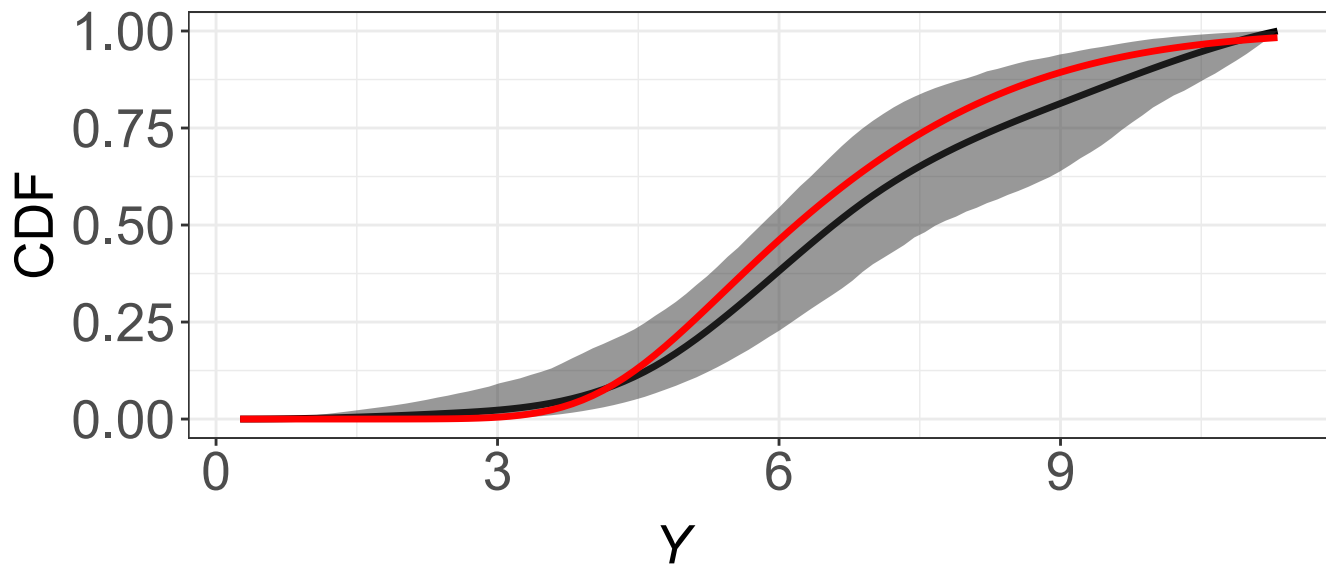

# Estimated Quantiles

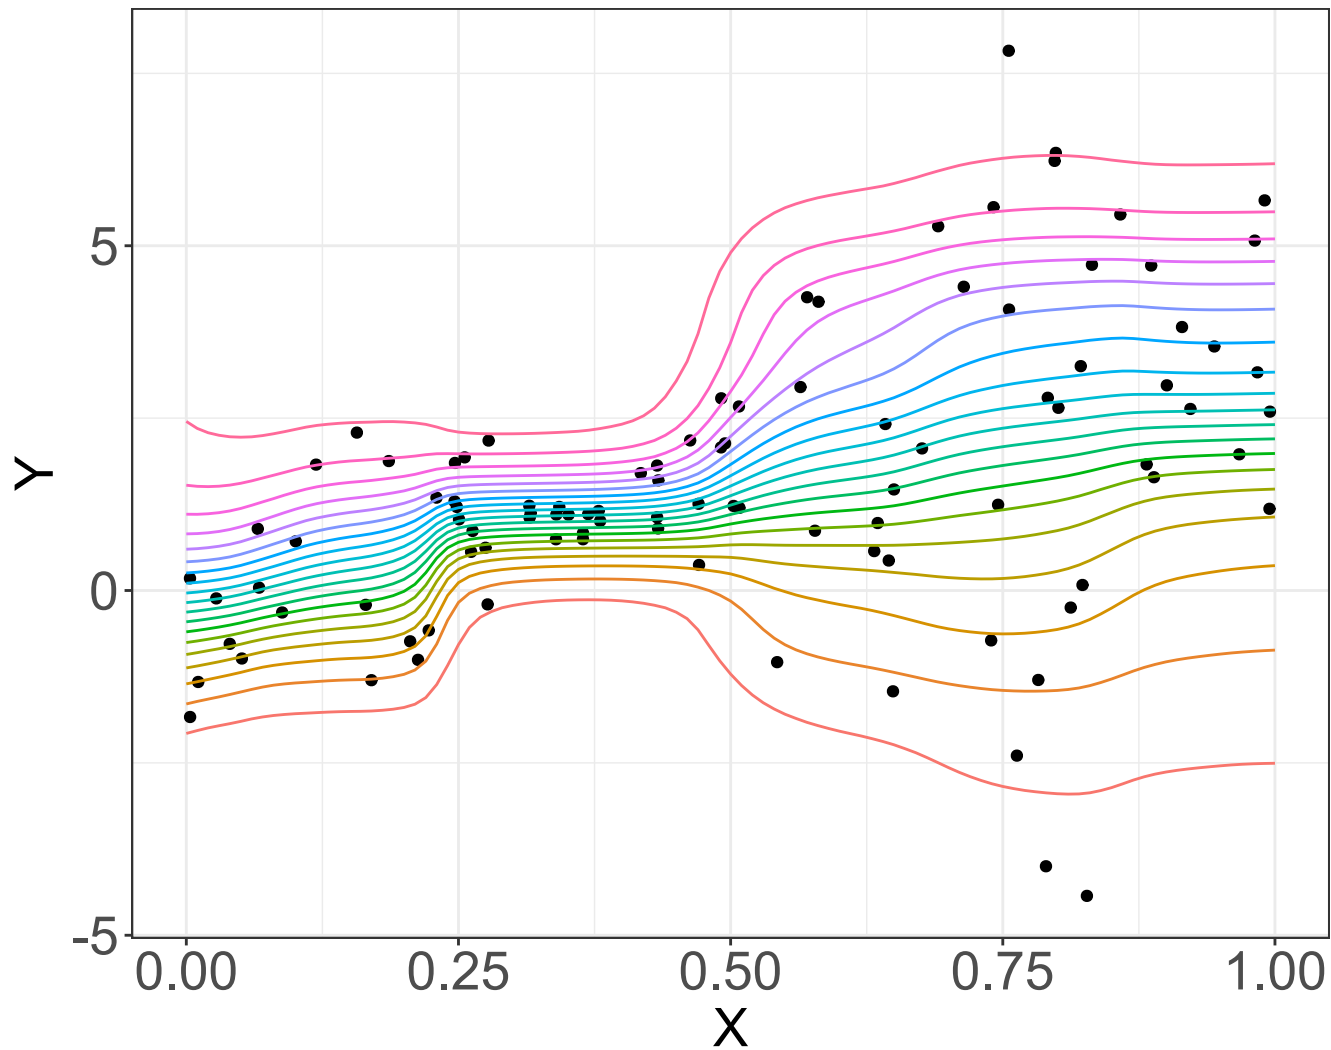

*Estimated Density at  $X = 0.15$*

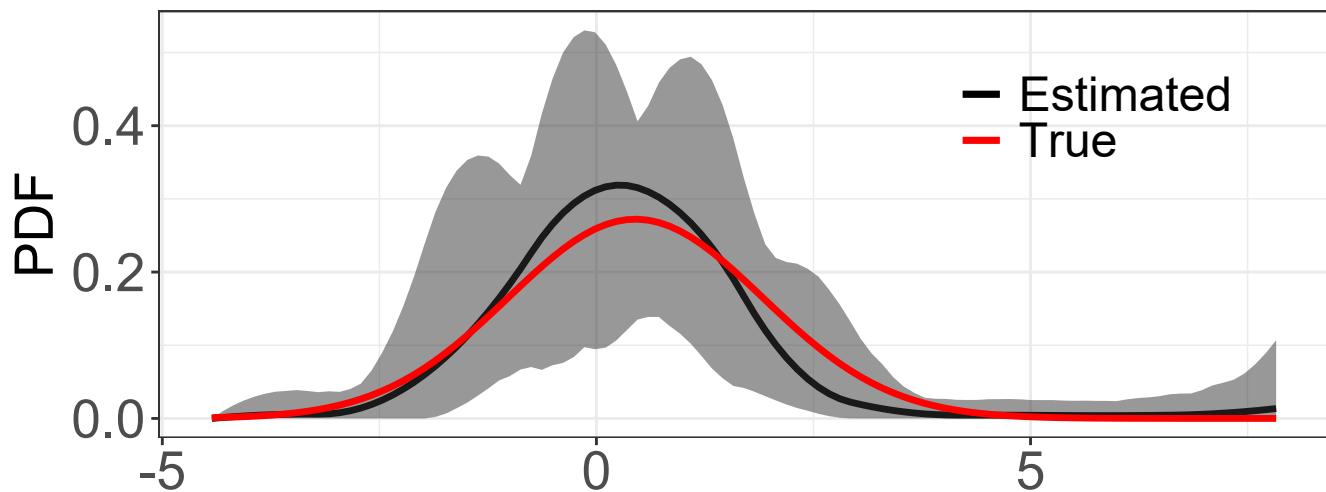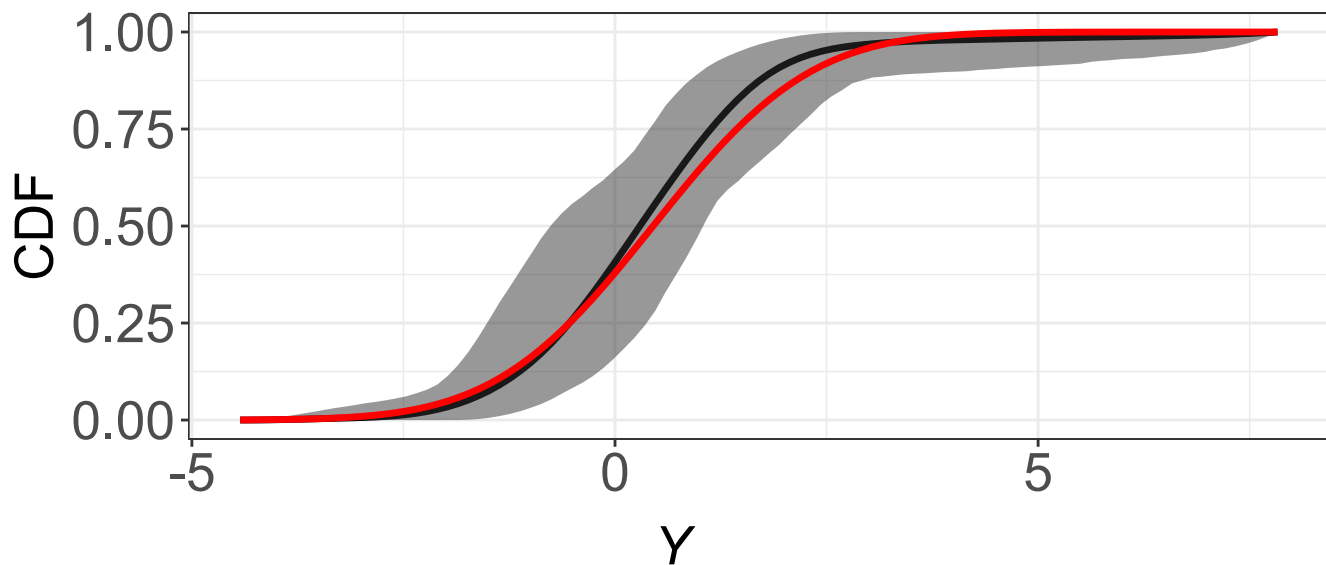



*Estimated Density at  $X = 0.5$*

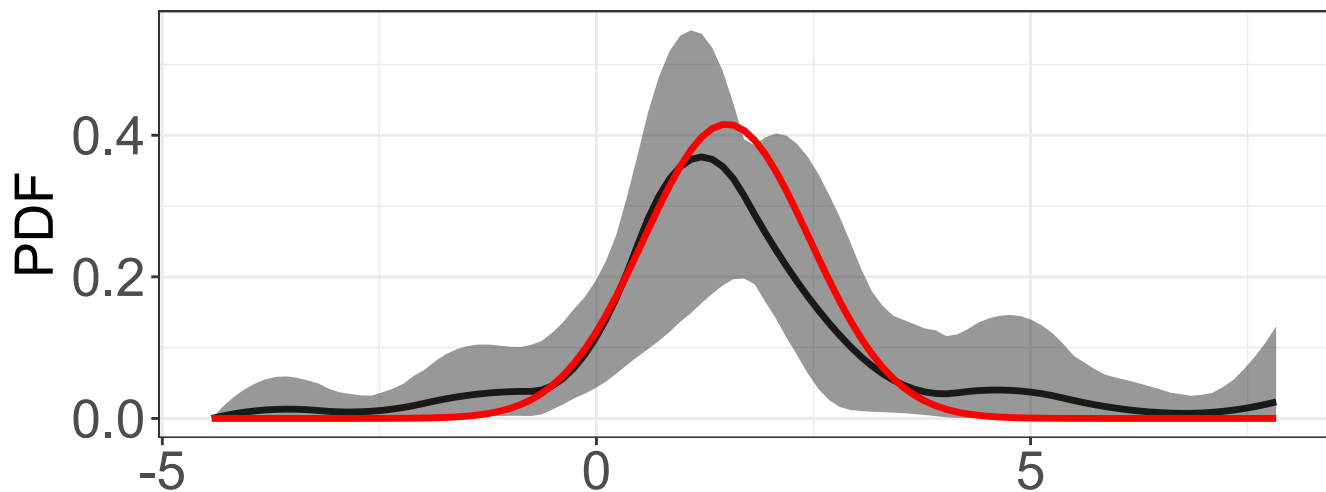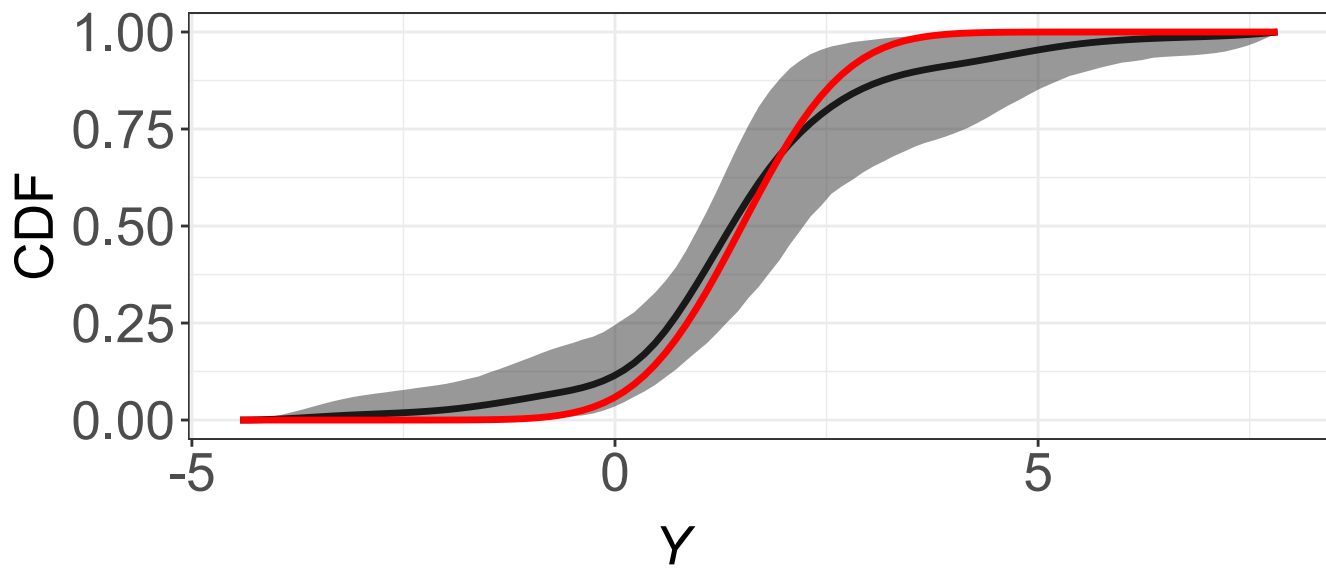

*Estimated Density at  $X = 0.7$*

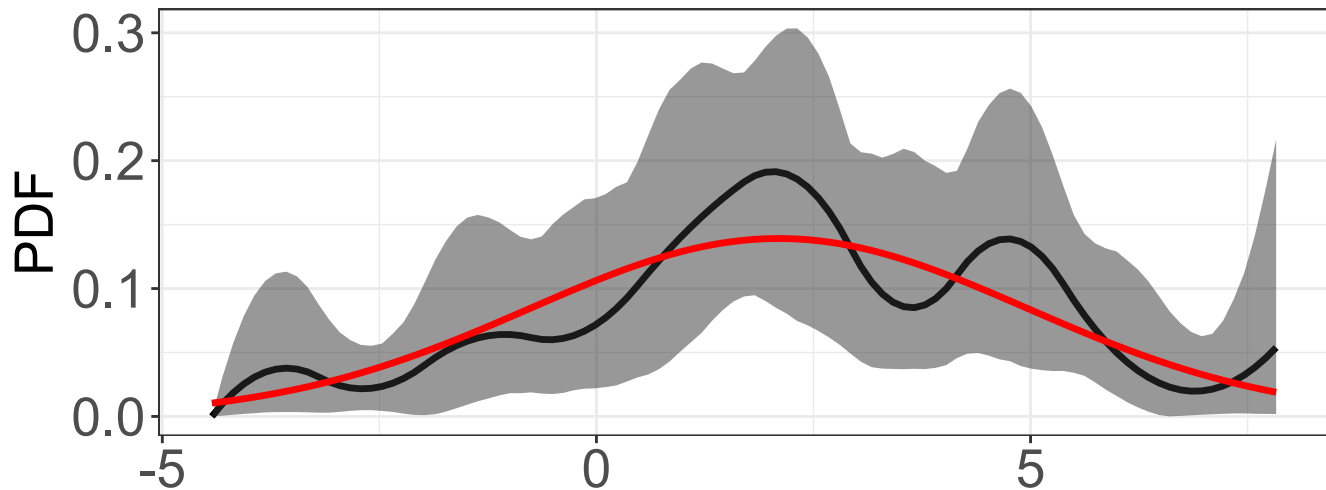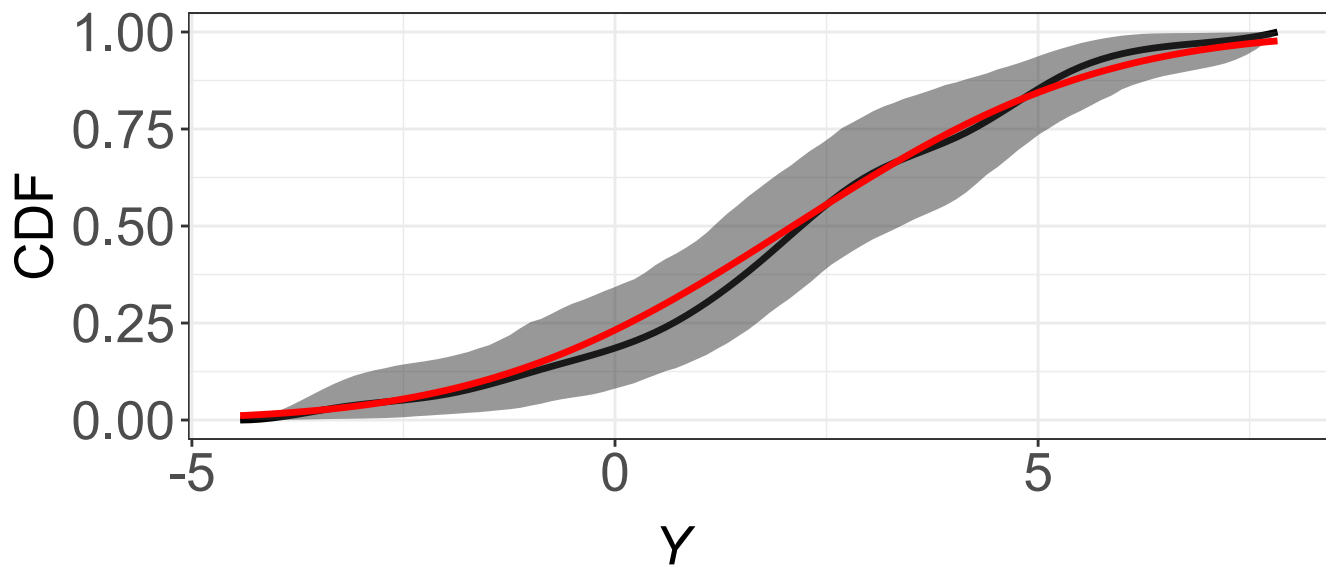

Supplement: Supplementary file 1 [file supp_simulation.pdf]
